# Supplementary material for: On Fairness of Medical Image Classification with Multiple Sensitive Attributes via Learning Orthogonal Representations
Source: arXiv:2301.01481 source file (2023-03-08)
Supplement: Supplementary file 1 [file appendix.tex]

\section*{Appendix}
\subsection*{Low-Rank Space Accumulation}\label{app:accu}
Here we describe how to construct $\wt{\mathcal{S}}_A$ iteratively with mini-batch data. At the first iteration, we initialize $\wt{\mathcal{S}}_A^{0}$ using SVD as introduced in Section~\ref{sec:space}. For the following $t$-th iteration, we first evaluate the importance of the $i$-th base $u_{A,i}^{t-1}$ in old space $\wt{\mathcal{S}}_A^{t-1}$ on the new representation matrix $Z_A^t$ with its corresponding eigenvalues $\delta_i^t=(u_{A,i}^{t-1})^\top Z_A^t(Z_A^t)^\top u_{A,i}^{t-1}$. Then we apply SVD to $\disp Z_A^t=Z_A^t-\wt{\mathcal{S}}_A^{t-1}(\wt{\mathcal{S}}_A^{t-1})^\top Z_A^t$ and get a set of new bases with singular values $\{\sigma^t_j\}$. Finally, we concatenate $\{\delta_i^t\}$ and $\{(\sigma^t_j)^2\}$ and sort them in a descending order. We take the top-half concatenated bases as $\wt{\mathcal{S}}_A^t$. This accumulation process lasts for 3 epochs, and we pick the top-$k$ bases as our final $\wt{\mathcal{S}}_A$.
